# Supplementary material for: Priority-Aware Model-Distributed Inference at Edge Networks
Source: arXiv:2412.12371 source file (2024-12-16)
Supplement: Supplementary file 1 [file Appendix.tex]

\noindent \textbf{\Large Appendix A}

\noindent \textbf{Network Utility Maximization (NUM) Formulation.}
Assume that images are arriving to the source node $\eta_i$ with rate $x_i$, which is associated with a utility function $g(x_i)$. Our MS-MDI algorithm described in Section \ref{sec:multi-AR-MDI} is designed based on the structure of the following NUM problem. 
\begin{align} \label{eq:NUMproblem} 
   \max & \sum_{\eta_i \in \Sset} g(x_i) \nonumber \\
   \text{s.t.~~} & x_i \leq x_i^l + x_i^d, \text{~} \forall \eta_i \in \Sset \nonumber \\ 
    & x_i^l \leq f_l^i, \text{~} \forall \eta_i \in \Sset \nonumber \\ 
    & f_{(n-1)\%N}^i + x_i^d 1_{[\eta_i \in \Sset]} \leq f_n^i, \text{~} \forall \eta_n \in \Nset, \forall \eta_i \in \Sset \nonumber \\
    & \mathbf{f} \in \Gamma, 
\end{align} where the rate $x_i$ is splitted into $x_i^l$; data that will be processed locally, and $x_i^d$; data that will be processed in a distributed manner. The first constraint in (\ref{eq:NUMproblem}) is the flow conservation constraint, which guarantees that the arriving data $x_i$ is not larger than the sum of the data that is processed locally $x_i^l$ and distributedly $x_i^d$. The second constraints makes sure that the data arriving for processed locally, \ie $x_i^l$ is less than the actual processing rate $f_l^i$ locally by the source node $\eta_i$. The third constraint is the flow conservation constraint for MDI, where $f_n^i$ is the rate of processed data at node $\eta_n$ for source node $\eta_i$, $1_{[\eta_i \in \Sset]}$ is an indicator function that takes a value of 1 if $\eta_i \in \Sset$, and becomes 0 if $\eta_i \notin \Sset$. Thus, if a node $\eta_n$ is a source device, it needs to process $x_i^d$ amount of data. Otherwise, it will receive data from the previous node $(n-1)\%N$ with rate $f_{(n-1)\%N}^i$. Eventually, the sum of $f_{(n-1)\%N}^i$ and $x_i^d 1_{[\eta_i \in \Sset]} \leq f_n^i$ should be less than the processing rate at node $\eta_n$ for source $\eta_i$. The last contraint makes sure that the vector of all processing rates $\mathbf{f}$ is in the supporting region of the system $\Gamma$, which is characterized by both the computing and communication cost of the system. 

\noindent \textbf{NUM Solution.} In this section, we provide a solution to the NUM problem in (\ref{eq:NUMproblem}) via Lagrange relaxation. By relaxing the first three constraints via Lagrange multipliers $\mu_i$, $q_l^i$, and $q_n^i$, respectively, we obtain the following Lagrange function
\begin{align} \label{eq:Lagrange1}
    L(\mathbf{x}, \mathbf{\mu}, \mathbf{q}) = & \sum_{\eta_i \in \Sset} g(x_i) - \sum_{\eta_i \in \Sset} \mu_i (x_i - x_i^d - x_i^l) - \nonumber \\
    & \sum_{\eta_i \in \Sset} q_l^i(x_i^l - f_l^i) - \sum_{\eta_i \in \Sset} \sum_{\eta_n \in \Nset} q_n^i (f_{(n-1)\%N}^i + \nonumber \\
    & x_i^d 1_{[\eta_i \in \Sset]} - f_n^i)
\end{align} where $\mathbf{x}$, $\mathbf{\mu}$, and $\mathbf{q}$ are vectors of $\mathbf{x} = \{x_i\}_{\forall \eta_i \in \Sset}$, $\mathbf{\mu} = \{\mu_i\}_{\forall \eta_i \in \Sset}$, $\mathbf{q} = \{q_n^i\}_{\forall \eta_i \in \Sset, \ \eta_n \in \Nset}$. 

The Lagrange function in (\ref{eq:Lagrange1}) is expressed as 
\begin{align}\label{eq:Lagrange2}
    L(x, \mu, q) = & \sum{\eta_i \in \Sset} (g_i(x_i) - \mu_ix_i) + \sum_{\eta_i \in \Sset} x_i^l(\mu_i - q_l^i) + \nonumber \\
    & \sum_{\eta_i \in \Sset} x_i^d(\mu_i - q_i^i) + \sum_{\eta_n in \Nset} q_l^n f_l^n + \nonumber \\
    & \sum_{\eta_j \in \Sset} \sum_{\eta_n \in \Nset} f_n^j (q_n^j - q_{(n+1)\%N}^j )
\end{align}
Assuming that $q_l^n(t) = 0$ if $\eta_n \notin \Sset$, (\ref{eq:Lagrange2}) is expressed as
\begin{align}
     L(x, \mu, q) = & \sum_{\eta_i \in \Sset} (g_i(x_i) - \mu_ix_i) + \label{eq:resor} \\
     & \sum_{\eta_i \in \Sset} ( x_i^l(\mu_i - q_l^i) + x_i^d(\mu_i - q_i^i))  + \label{eq:queueIns} \\
     & \sum_{\eta_n \in \Nset} (q_l^nf_l^n + \sum_{\eta_j \in \Sset} f_n^j (q_n^j - q_{(n+1)\%N}^j) ) \label{eq:dataXmit}
\end{align} Our algorithm described in Section \ref{sec:multi-AR-MDI} is designed based on the maximization of the Lagrange function described in (\ref{eq:resor})-(\ref{eq:dataXmit}). As seen, the Lagrange function is decomposed into three parts, which corresponds to our policies as explained next. 

%maximization solutions in (\ref{eq:resor}), (\ref{eq:queueIns}), and (\ref{eq:dataXmit}), which we explain in detail next. 

The data arrivals in our system is according to Poisson arrival, so when an image is collected at source worker $\eta_i$, it is inserted in reservoir queue $\mu_i$. We note that it is straightforward to extend our algorithm to maximize $(g_i(x_i) - \mu_ix_i)$ at source worker $\eta_i$, where images could be collected to maximize the utility function $g_i(x_i)$.

Our policy of inserting data in a queue that satisfies $\min \{q_l^i(t), q_i^i(t)\}$ is designed based on (\ref{eq:queueIns}), which reduces to our policy if inserting data to only one queue is allowed at slot $t$. Our policy of selecting queues for inference (\ref{eq:policy2}) is designed based on the  solution of (\ref{eq:dataXmit}) if only one queue is updated at slot $t$. 

~

% \noindent \textbf{\Large Appendix B} 

% \begin{table}[t!]
% \vspace{10pt}
% \centering
% \caption{Notation table.}
% \label{table:notation}
% \begin{tabular}{|l|c|}
% \hline
%   MDS   & 4       \\ \hline
% Repetition   &  $3\lfloor \frac{N}{4}\rfloor+1$     \\ \hline
% \end{tabular}
% \vspace{-5pt}
% \end{table}
